# Supplementary material for: Macro2Micro: A Rapid and Precise Cross-modal Magnetic Resonance Imaging Synthesis using Multi-scale Structural Brain Similarity
Source: arXiv:2412.11277 source file (2025-10-25)
Supplement: Supplementary file 1 [file Supplementary__draft_.tex]

The total intelligence score in the NIH toolbox was used for the intelligence prediction task. The parent KSAD (Kiddie Schedule for Affective Disorders and Schizophrenia) was employed as the diagnostic tool for assessing ADHD in children. Children who did not receive a diagnosis of KSAD and obtained a total problem score below 65 on the Child Behavior Checklist (CBCL) were designated as the healthy control group. We assessed the accuracy of classification tasks using FA images generated by CycleGAN, Pix2Pix, and Macro2Micro.

Additionally, we compared the predictive performance of these generated FA images with ground truth FA images or T1 images. Logistic regression with L2 norm was employed for gender classification, and PCA was used as the feature extraction method. PCA was applied to flattened, background-removed brain features, and feature reduction was performed by selecting the top 1,000 components (sex) and 500 components (Total intelligence, ADHD) that accounted for more than 90\% of the explained variance. The analysis was conducted on the test dataset of the image generation task. Among these datasets, 20\% were held out as a test set, while the remaining 80\% of the subjects were used for a training set in a 5-fold cross-validation. The models trained on these five folds were used to evaluate the performance on the held-out test set, and the results were averaged. Accuracy and AUROC were utilized for evaluating performances in classification tasks. Pearson product-moment correlation coefficients and mean square error (MSE) were chosen for evaluating the regression task.

\input{Table/norm_relu}

\textbf{Normalization \& Activation Function.}
Normalization and activation functions affect the quality of the generated images. In Table~\ref{tab:norm_relu}, we found that the normalization including batch normalization or instance normalization, and the ReLU activation function don't aid our Macro2Micro in synthesizing high-quality images. The combination of not using normalization and using leaky ReLU as an activation function performs the highest SSIM and PSNR scores and the lowest MAE and MSE scores. Also, the results using normalization or ReLU function have artifacts like dotted lines at the borders of the brain (Figure~\ref{fig:norm_relu}).
